# Supplementary material for: A Game-theoretic Approach for Provably-Uniform Random Number Generation in Decentralized Networks
Source: arXiv:2309.11250 source file (2023-09-20)
Supplement: Supplementary file 1 [file appendix1.tex]

%!TEX program = xelatex
%!TEX root = ./thesis.tex
\chapter{Appendix 1}
